# Supplementary material for: Trajectory Optimization for Adaptive Informative Path Planning with Multimodal Sensing
Source: arXiv:2404.18374 source file (2024-04-29)
Supplement: Supplementary file 1 [file 6_Appendix.tex]

\subsection{Descent Step Size} While several methods have been proposed for step size selection in descent-based optimization, backtracking line search has been a popular choice in the projection-based trajectory optimization literature \cite{miller2013trajectory, dressel2018efficient}. The candidate step size is initialized to $\gamma_0$ and multiplied by a constant $\tau \in (0,1)$ at each iteration. The process terminates when the first Wolfe condition is satisfied \cite{kochenderfer2019algorithms}: \begin{equation}
\begin{aligned}
    & J(\mathscr{P}(\tilde{x}_{0:T} + \gamma z_{0:T}, \tilde{u}_{0:T} + \gamma v_{0:T}, x_0)) \leq J(\tilde{x}_{0:T},\tilde{u}_{0:T})  \\ 
    & \hspace{5em} + \rho \gamma \nabla J(\tilde{x}_{0:T}, \tilde{u}_{0:T}) \cdot (z_{0:T}, v_{0:T}) 
\end{aligned}
\end{equation} where $\rho \in (0,1)$ is the first Wolfe parameter and $\mathscr{P}(\cdot)$ is the projection operator.

\subsection{Riccati Gain}
The gains $\mathscr{K}_t$ come from a linear quadratic regulator (LQR) problem. In the case of nonlinear dynamics, the projected trajectory will deviate from the reference candidate trajectory and we would like to minimize these deviations as much as possible. Let $\delta \tilde{x}_t$ and $\delta \tilde{u}_t$ represent deviations from the candidate trajectory and control at time step $t$, we can then write the following LQR problem: \begin{align}
& \underset{\delta \tilde{x}_t,\delta \tilde{u}_t}{\text{minimize}} \sum_{t=0}^T \Bigl(\delta \tilde{x}_t^T Q_n \delta \tilde{x}_t + \delta \tilde{u}_t^T R_n \delta \tilde{u}_t \Bigr) \nonumber \\
& \text{subject to}  \hspace{1em} \delta \tilde{x}_{t+1} = \tilde{A}_t\delta \tilde{x}_t + \tilde{B}_t \delta \tilde{u}_t \nonumber \\
& \hspace{5em} \delta \tilde{x}_0 = \mathbf{0}. \end{align}The gains are then computed with a Riccati-like backwards iteration \cite{miller2013trajectory, dressel2019tutorial}: 
$$P_T = Q_n$$
$$r_T = a_T$$
$$\Gamma_t = R_n + \tilde{B}_t^T P_{t+1} \tilde{B}_t$$
$$\mathscr{K}_t = \Gamma_t^{-1}\tilde{B}_t^TP_{t+1}\tilde{A}_t$$
$$P_t = Q_n + \tilde{A}_t^TP_{t+1}\tilde{A}_t -\mathscr{K}_t^T \Gamma_t \mathscr{K}_t$$
$$r_t = a_t + (\tilde{A}_t^T - \mathscr{K}_t^T \tilde{B}_t^T) r_{t+1} - \mathscr{K}_t^T b_t.$$ As noted by Dressel et al. if the system dynamics are linear, the candidate trajectory will be feasible because the descent problem uses linearized dynamics \cite{dressel2019tutorial}. 

\subsection{Budget Constraint}
Initial trajectory selection: our approach begins with an initial trajectory that inherently adheres to the budget constraint. To ensure feasibility, we adopt the shortest path to the goal as this initial trajectory. This choice not only provides a practical starting point but also guarantees our trajectory optimization process starts from a budget-compliant state.

Control input limitation: during the optimization process, the control inputs, denoted as $u_t$, are constrained such that they cannot push the trajectory beyond the permissible budgetary limit. Even if the optimization's descent direction suggests a trajectory that might potentially exceed the budget, the limitation on $u_t$ ensures that the budget is never breached. Conceptually, this can be thought of as distributing the budget evenly across the trajectory, and ensuring that at each step, we never draw more than is allowed by the budget constraint.

Managing random perturbation samples: in situations where random perturbation samples are integrated, particularly using the InjectSamples() function detailed in Algorithm 1, a trajectory that surpasses the budgetary allowance necessitates truncation. This shortening inherently influences the sensing strategy – as the trajectory length (and thus potential measurement locations) decreases, the system has to judiciously balance between the number and the precision of sensor measurements. This induces a trade-off between the quantity and quality of sensing, enforcing the system to operate within the set budget.

\subsection{Additional Experiments}
We also evaluated our proposed method with several other variations that we will describe here to highlight the flexibility of our approach. 
\subsubsection{True Map Sampled from Gaussian Process}
It is important to note that the true map of the environment shown in Figure \ref{fig:all_trajectories} is a grid-like environment that is out of the distribution of the Gaussian process belief. For further comparison, we also evaluated our method on true maps that were sampled from a Gaussian process and the results are shown in Figures \ref{fig:ae_all_trajectories} and \ref{fig:ae_trace_rmse}. As expected, these smoother varying maps that are more aligned with the Gaussian process kernel function result in lower RMSE values.

\subsubsection{Larger Map Sizes}
To highlight the scalability of our proposed approach, we have also included an example trajectory from our GP-PTO method with a true map of size $640 \times 640$ consistent with the size used by Arora et al. \cite{arora2019multi}. During the optimization, the Gaussian process is queried at a fixed number of locations to evaluate the variance, expected improvement, or any other information-theoretic metric. Additionally, since the GP-PTO method has a continuous action space, we are not constrained by the size of the map and therefore the number of query points can be varied based on computational requirements. These results are shown in Figure \ref{fig:ae_large_map}. 

\begin{figure*}[t]
\centering
    {\includegraphics[width=1.0\textwidth]{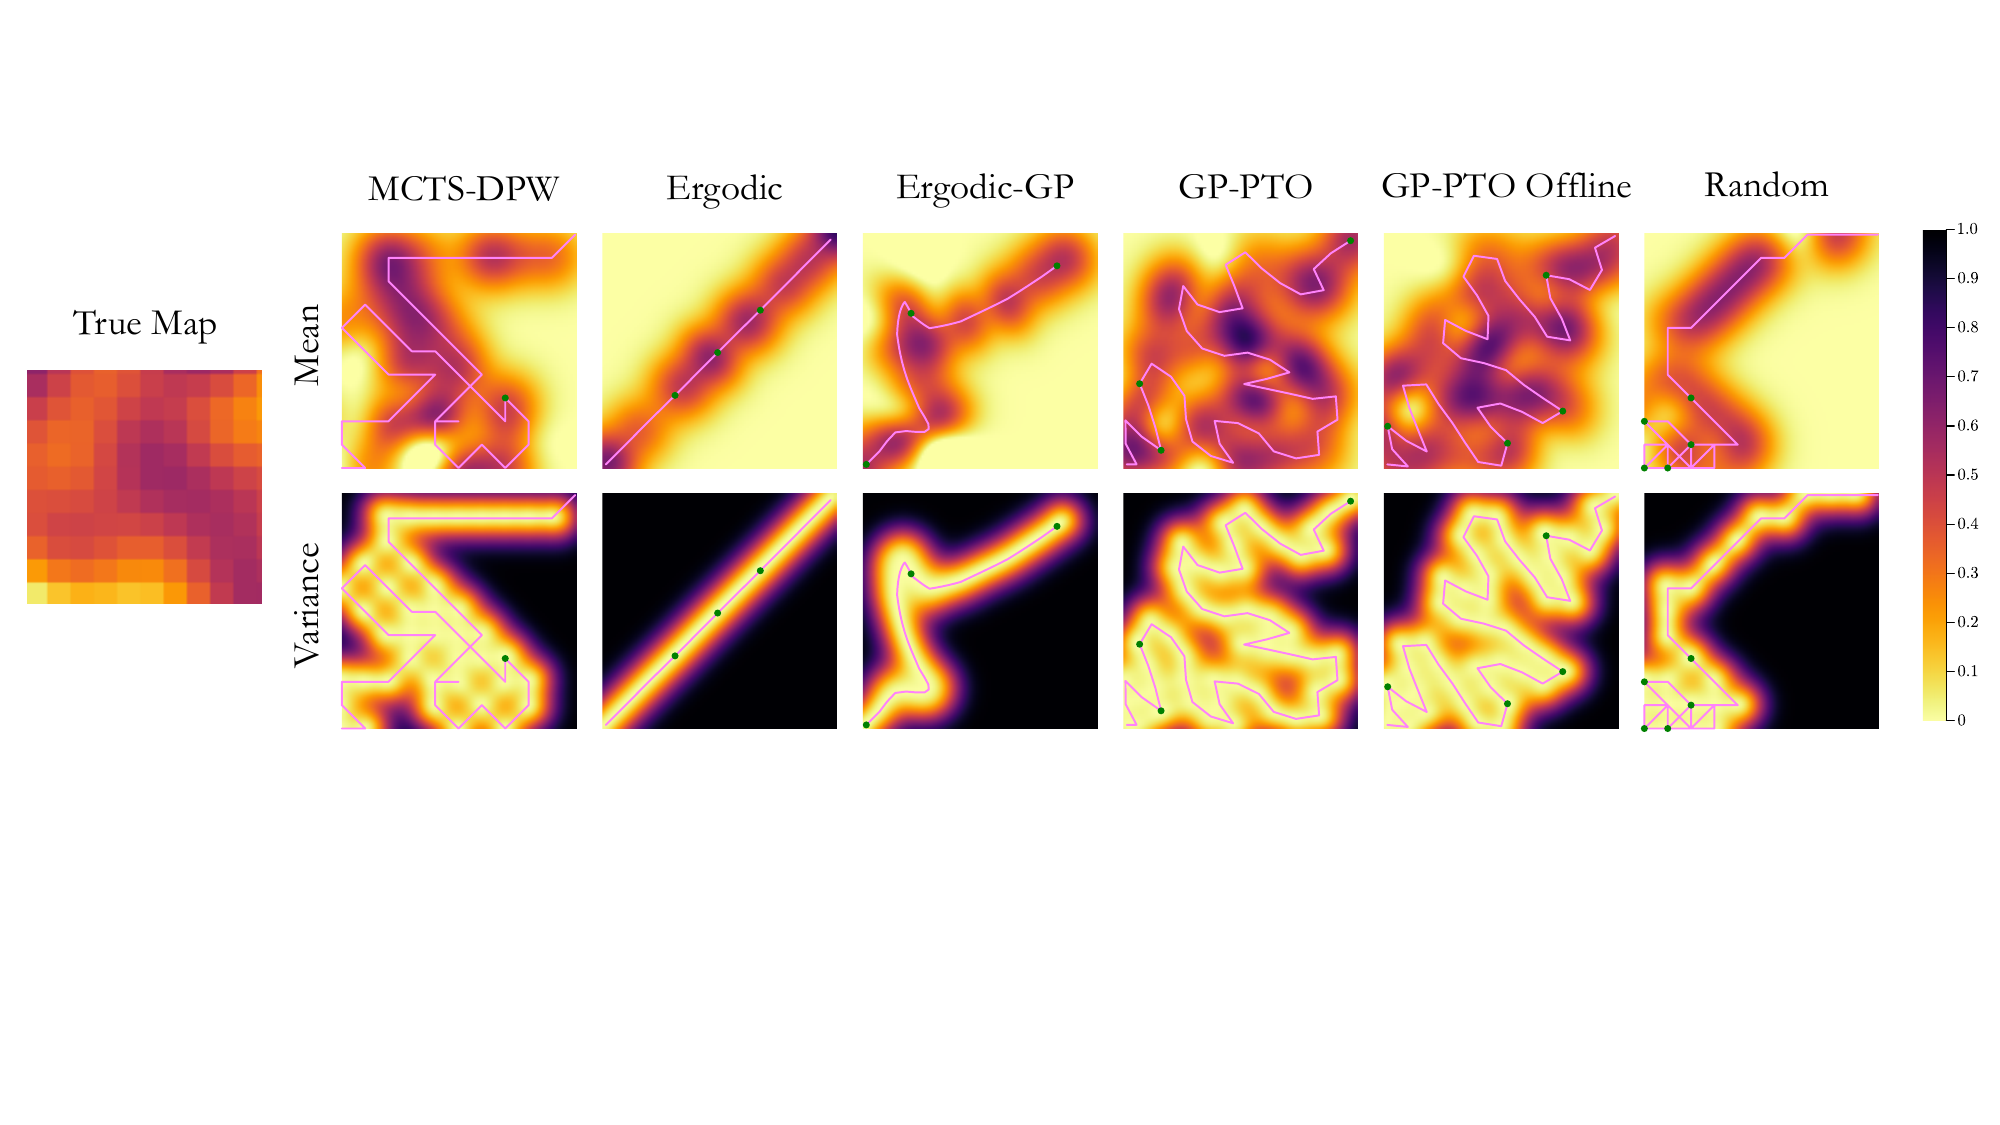}}
  \caption{Examples of trajectories produced from each of the six methods considered in this work. The true map is sampled from a Gaussian process and is shown on the left. These trajectories were generated with $\sigma_s = 0.1$ and $b = 60.0$.} 
  \label{fig:ae_all_trajectories}
\end{figure*}

\begin{figure*}[t]
\centering
    {\includegraphics[width=0.750\textwidth]{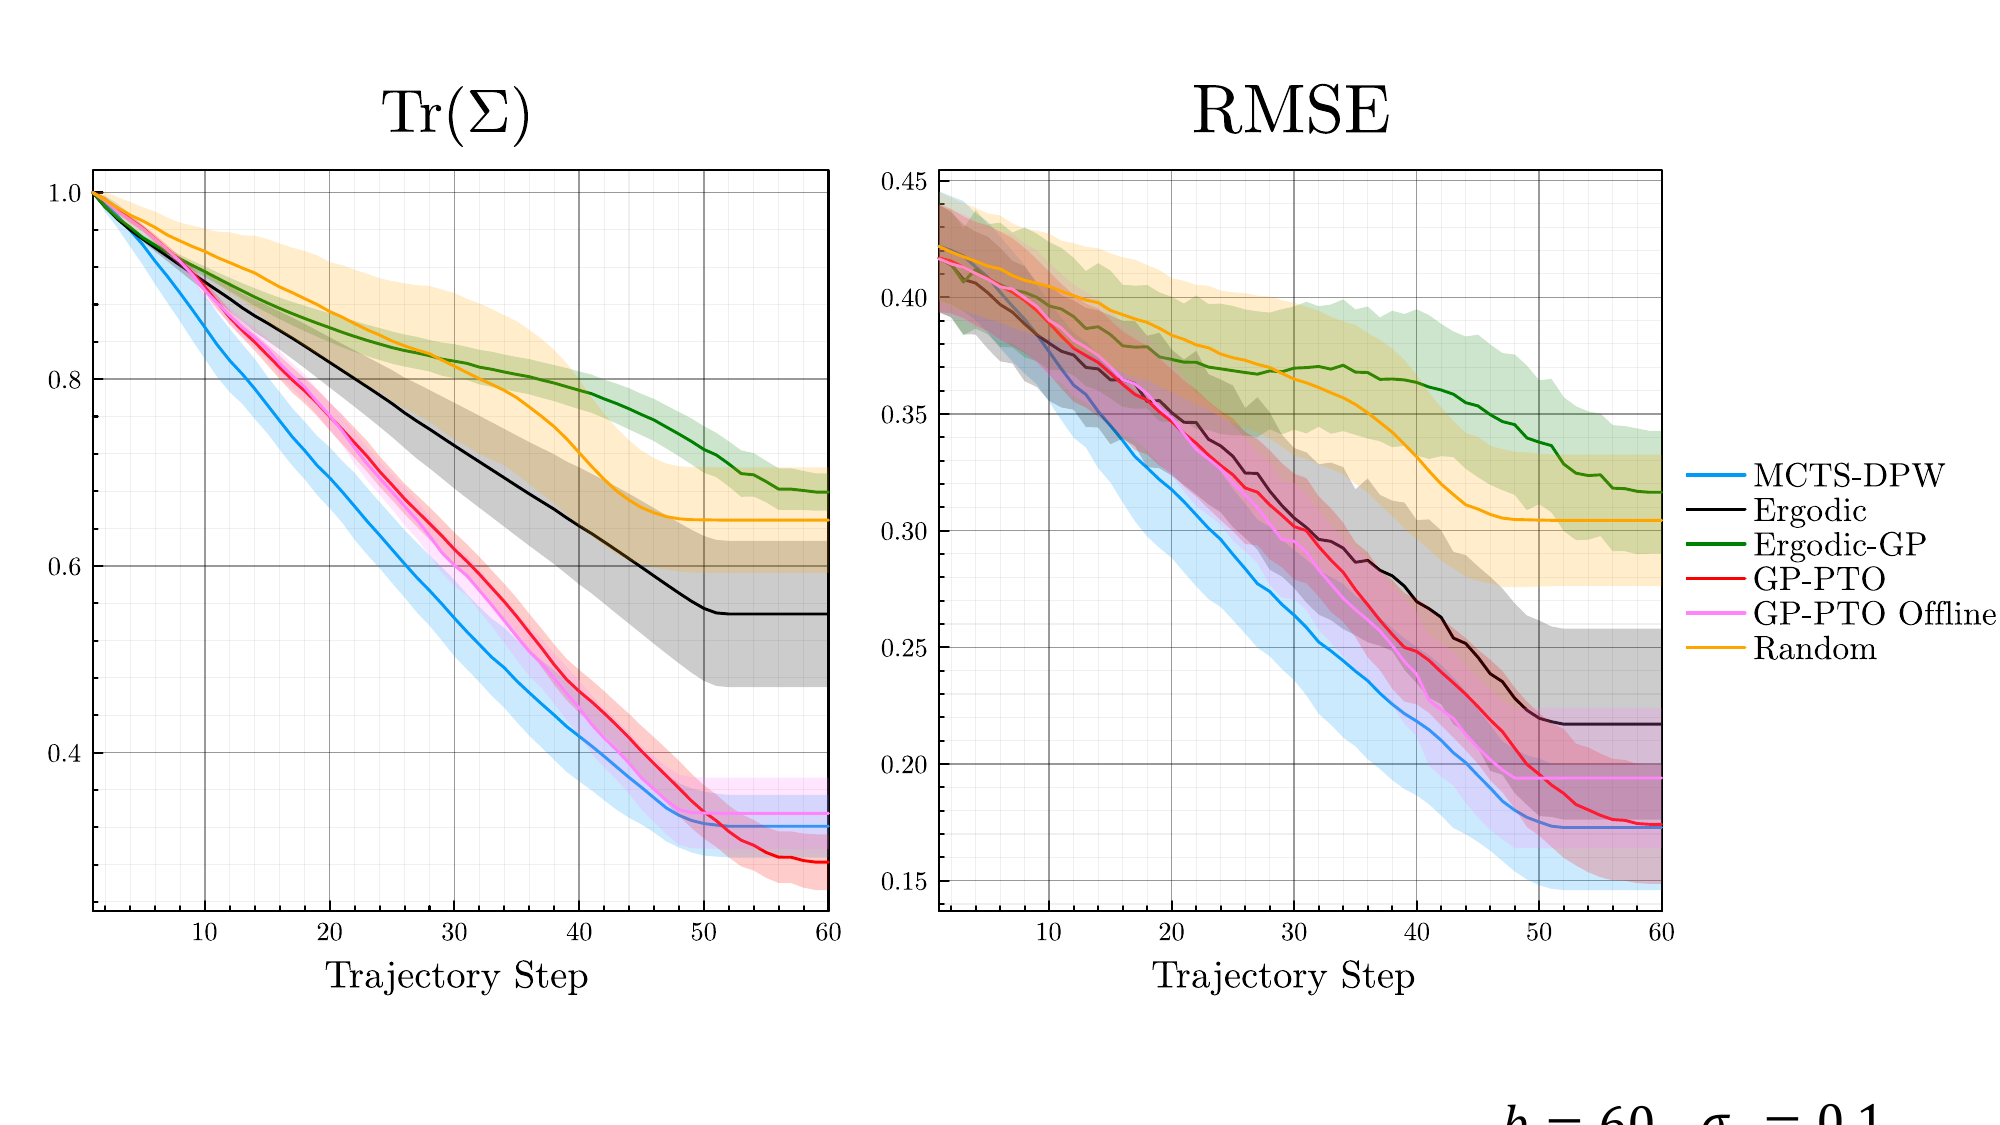}}
  \caption{Trace and RMSE results with respect to the true map when the true map is sampled from a Gaussian process. The average and standard deviation from 50 simulation runs are shown with a budget of $b=60$ and spectrometer noise of $\sigma_s = 0.1$.} 
  \label{fig:ae_trace_rmse}
\end{figure*}

\begin{figure*}[t]
\centering
    {\includegraphics[width=1.0\textwidth]{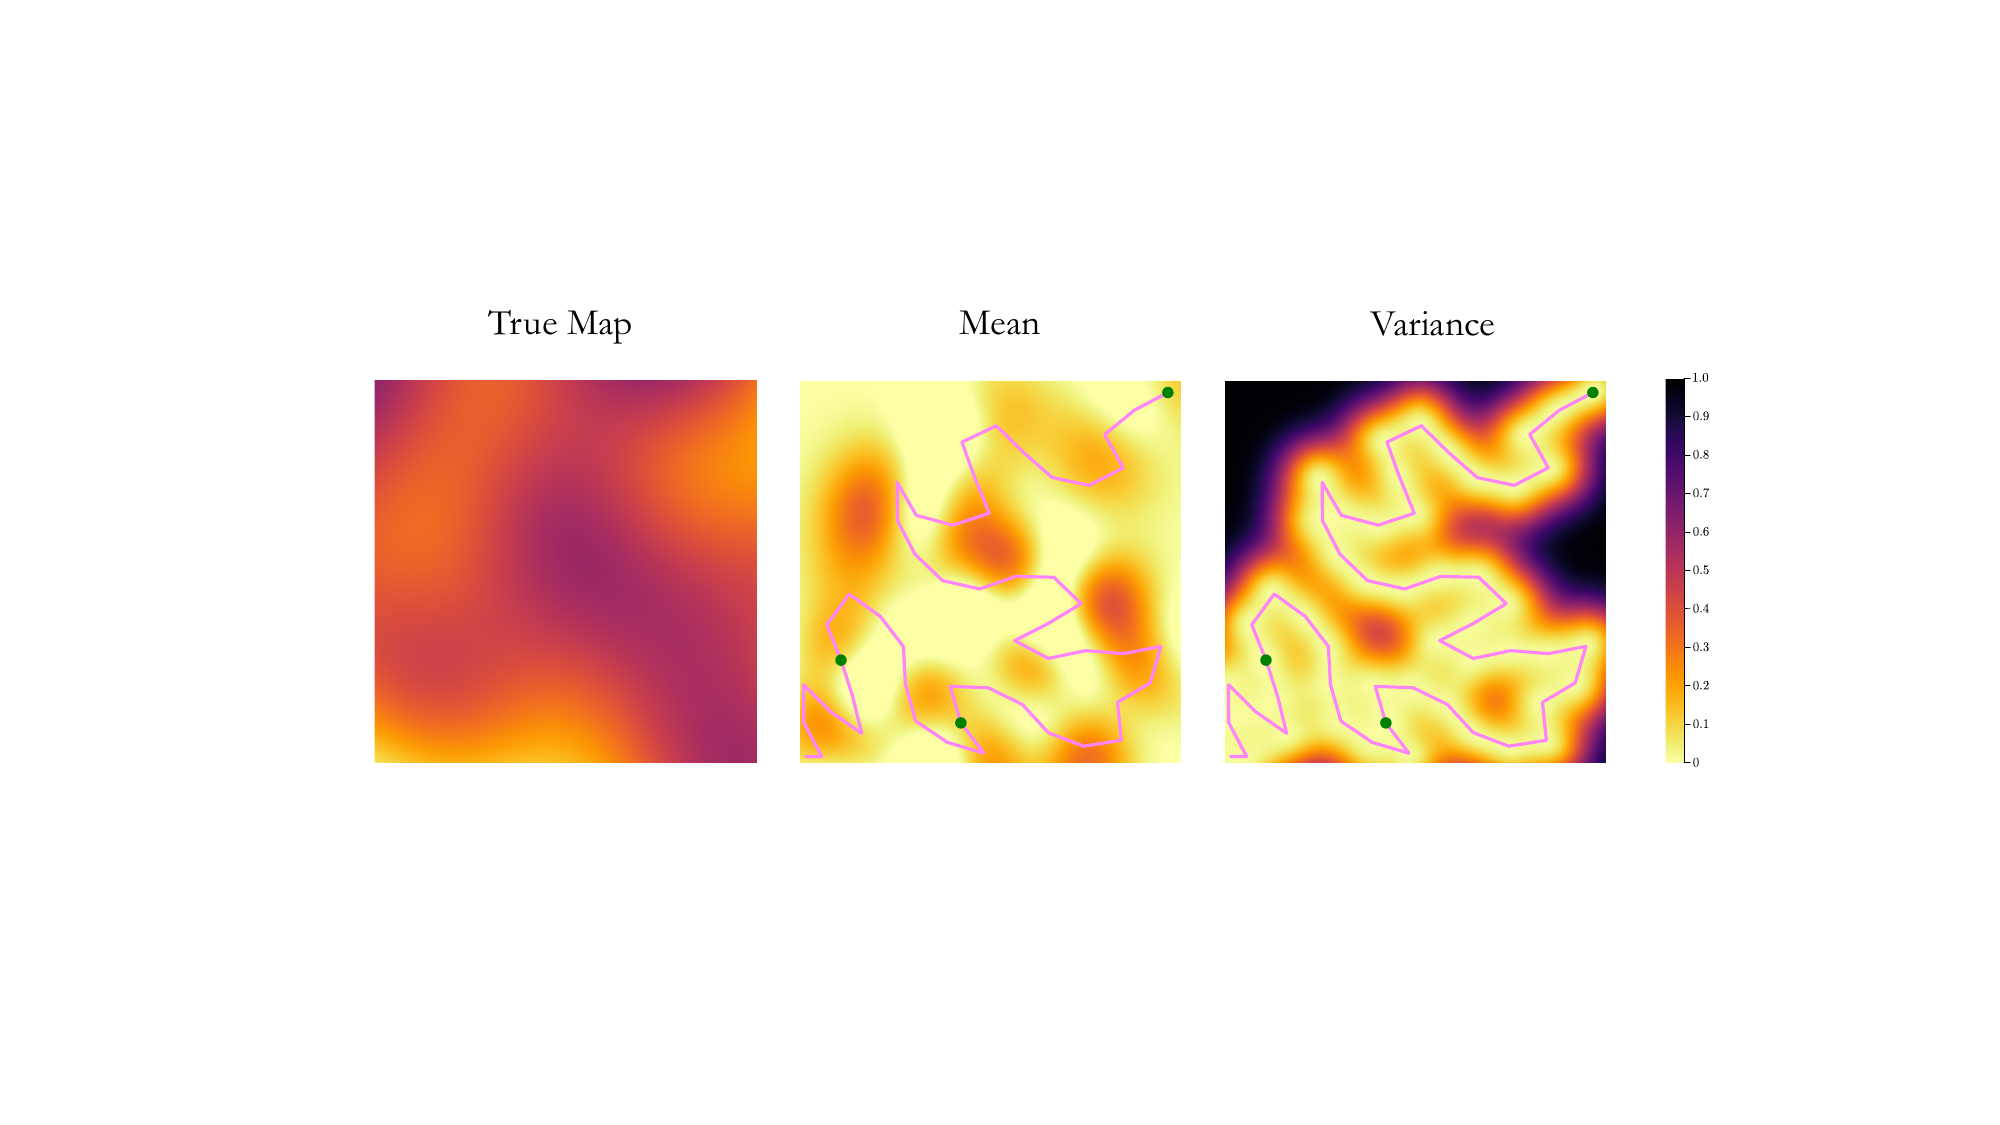}}
  \caption{GP-PTO result where the true map is of size $640 \times 640$.} 
  \label{fig:ae_large_map}
\end{figure*}

\newpage
\begin{algorithm}
\caption{Trajectory Optimization for Adaptive Informative Path Planning with Multimodal Sensing}\label{alg:cap}
\begin{algorithmic}
\State \textbf{Initialize}
\State $x_{0:T}, u_{0:T}$ \Comment{initial state and control input trajectory}
\State $M_0$ \Comment{initial sample locations \& measurement type}
\State $\gamma_0$, $\tau$, $\rho$ \Comment{initial step size, decay, and Wolfe parameter}
\State $p$ \Comment{probability of injecting new sample}
\\
\Function{Linearize}{$f$, $x_{t}$, $u_{t}$}
  \NoDo
  \State $A_t \leftarrow \nabla_x h(x_t, u_t)$
  \State $B_t \leftarrow \nabla_u h(x_t, u_t)$
  \State \Return $A_t, B_t$
\EndFunction
\\

\Function{$\mathscr{P}$}{$\Omega_{0:T}, \tilde{\alpha}_{0:T}$, $\tilde{\mu}_{0:T}$, $x_0$}
  \NoDo
  \State $\mathscr{K}_{0:T} \leftarrow \textsc{SolveRiccati}(\Omega_{0:T})$
  \For $t \in 0:T-1$
      \State $\tilde{u}_t \leftarrow \tilde{\mu}_t+\mathscr{K}_t\left(\tilde{\alpha}_t -\tilde{x}_t\right)$
      \State $\tilde{x}_{t+1} \leftarrow \tilde{x}_t + f\left(\tilde{x}_t, \tilde{u}_t\right) \Delta t$    
  \EndFor
  \State \Return $\tilde{x}_{0:T}, \tilde{u}_{0:T}$
\EndFunction
\\

\Function{LineSearch}{$\Omega, z, v, x, u$}
  \NoDo
  \State $\tilde{\alpha} \leftarrow x + \gamma z$
  \State $\tilde{\mu} \leftarrow u + \gamma v$
  \State $\eta \leftarrow \rho \gamma \nabla J(x, u) \cdot (z, v)$
  \While $J(\mathscr{P}(\Omega, \tilde{\alpha}, \tilde{\mu}, x_0)) \leq J(x,u) + \eta $
  \State $\gamma \leftarrow \tau \gamma $
  \State $\eta \leftarrow \rho \gamma \nabla J(x, u) \cdot (z, v)$
  \EndWhile 
  \State \Return $\gamma$
\EndFunction
\\

\Function{InjectSamples}{$M_t, x_{0:T}, u_{0:T}$}
  \NoDo
   \If{$\text{rand()} < p$}
        \State $i = \text{rand(0:T)} $ %
        \State $\nu_i \leftarrow \textsc{PreturbSensorType}(\nu_i)$
        \State $x_{0:T}^{'}, u_{0:T}^{'}, M_t^{'} \leftarrow \textsc{Update}(x_{0:T}, u_{0:T}, M_t, \nu_i)$ %
        \If{$J(x_{0:T}^{'}, u_{0:T}^{'}, M_t^{'}) < J(x_{0:T}, u_{0:T}, M_t)$} 
            \State $x_{0:T}, u_{0:T}, M_t \leftarrow x_{0:T}^{'}, u_{0:T}^{'}, M_t^{'}$
        \EndIf
\EndIf
\State \Return $M_t$
\EndFunction

\\
\While \text{not converged}
    \For $t \in 0:T$
        \State $A_t, B_t \leftarrow \textsc{Linearize}$$(f$, $x_t$, $u_t)$ 
        \State $a_t \leftarrow \nabla_x J(x_t,u_t)$ 
        \State $b_t \leftarrow \nabla_u J(x_t,u_t)$
        \State $\Omega_t \leftarrow (A_t, B_t, a_t, b_t) $ %
    \EndFor
    \State $z_{0:T}, v_{0:T} \leftarrow \textsc{DescentDirection}(\Omega_{0:T})$
    \State $\gamma \leftarrow \textsc{LineSearch}(\Omega_{0:T}, z_{0:T}, v_{0:T}, x_{0:T}, u_{0:T})$
    \State $\tilde{x}_{0:T}, \tilde{u}_{0:T} \leftarrow \mathscr{P}(\Omega_{0:T}, x_{0:T}+\gamma z_{0:T}, u_{0:T}+\gamma v_{0:T}, x_0)$
    \State $M_t \leftarrow \textsc{InjectSamples}(M_t, \tilde{x}_{0:T}, \tilde{u}_{0:T})$
\EndWhile
\end{algorithmic}
\end{algorithm}
